# Supplementary material for: Automated Survey Collection with LLM-based Conversational Agents
Source: arXiv:2504.02891 source file (2025-04-02)
Supplement: Supplementary file 2 [file cover_letter.tex]

Dr. Nicholas Dobbins
Assistant Professor
Department of Biomedical Informatics \& Data Science
Johns Hopkins University
Baltimore, MA 21287
nic.dobbins@jhu.edu


April 29, 2024


Dr. Suzanne Bakken
Editor-in-Chief
Journal of the American Medical Informatics Association


Dear Dr. Bakken,

I am pleased to submit an original research article entitled "Towards Universal Model-Agnostic Federated Cohort Discovery" to be considered for publication in the Journal of the American Medical Informatics Association.

This manuscript describes the integration of i2b2, SHRINE, and Leaf, widely used cohort discovery applications applications at academic medical centers and research organizations around the world. We first explain our approach for integrating and translating queries and concepts, then evaluate by randomly selecting past SHRINE queries on the ACT network, translating them, and re-executing on 2 different data models, with the vast majority, 91.1\% of queries returning approximately the same results. Our work is, to the best of our knowledge, the first to demonstrate interoperability among such tools and robustly evaluate.

This manuscript has not been previously published and is not under consideration elsewhere. We have no conflicts of interest to disclose. Thank you for your consideration.

Sincerely,

Nicholas Dobbins, PhD, MLIS
